# Supplementary material for: CoTracker: It is Better to Track Together
Source: arXiv:2307.07635 source file (2024-10-01)
Supplement: Supplementary file 1 [file appendix.tex]

\appendix\section{Appendix --- scratch}

\subsection{Transformer and track correlation}

TODO: Give some details on the transformer and explain the kind of attention.

Appearance is coded by features We compute convolutional feature maps for all the frames of the current sliding window: $\phi_t = \phi(I_t) \in \mathbb{R}^{d\times \frac{H}{k} \times \frac{W}{k}}, k=8,  1 \leq t \leq S$.

Note that tracks are not defined before their start time $t^i$; nevertheless, for processing uniformity, we define the track position $\hat P^i_t$ and visibility $\hat v^i_t$ for all values of $t$.

The input to our method is a video $V$ and a set of points $P$ that we wish to track in the video.
The video $V = (I_t)_{t=1}^T$ is a sequence of $T$ RGB frames $I_t \in \mathbb{R}^{3 \times H \times W}$ and $P$ is a collection of $N$ points
$
P_i = (x^i, y^i, t^i) \in \mathbb{R}^{3},
$
each of which specifies the starting location $(x^i, y^i)$ and time $t^i$ of a video track.
We assume that tracked points are visible at the beginning of the track.
Different tracks can start at different times, so that new tracks can be added as more points become visible.

The goal is to predict a corresponding set of tracks
$
\hat P_t^i = (x_t^i, y_t^i, v_t^i)
$
for all points $i=1,\dots,N$ and valid times $t=t^i,\dots,T$.

where
$
(\hat P_t^i)_{i=1,t=t^i}^{N,T}
$
specifies the location and visibility of point $i$ at time $t$.
Here $v_t^i \in \{0,1\}$ is a binary flag that denotes whether the point is visible in a given video frame or not.
Hence, by definition,
$
x_{t^i}^i = x^i
$,
$
y_{t^i}^i = y^i
$,
and
$
v_{t^i}^i = 1.
$

\paragraph{Sliding window inference.}

While our model can process reasonably long video sequence in a single application of the neural network predictor, for longer videos we resort to a sliding window approach.
Specifically, a video of length $T$ greater than a window size $S$ are split into overlapping windows of length $S$.
Two consecutive windows overlap by $S/2$ samples.with overlapping sliding windows of size $S\leq T$, with an overlap of size $\frac{S}{2}$. It takes predictions from the previous sliding window as input to the current window. 

\subsection{Architecture}\label{sec:architecture}

The model processes videos of length $T$ with overlapping sliding windows of size $S\leq T$, with an overlap of size $\frac{S}{2}$. It takes predictions from the previous sliding window as input to the current window. 

\paragraph{Image features}
We compute convolutional feature maps for all the frames of the current sliding window: $\phi_t = \phi(I_t) \in \mathbb{R}^{d\times \frac{H}{k} \times \frac{W}{k}}, k=8,  1 \leq t \leq S$.

\paragraph{Tracked features}
We bi-linearly sample feature maps $\phi_t$ with the \textit{queried point's coordinates} $(x_{t^i}^i, y_{t^i}^i)$ at the \textit{queried frame index} $t^i$ : $Q_i  = Sample\big (\phi_{t^i}, (x_{t^i}^i, y_{t^i}^i)\big ) \in \mathbb{R}^d$.  We sample feature maps only at the queried position and use them to track queried points across the whole video of length $T$.

\paragraph{Iterative updates}
The model iteratively updates trajectory and visibility estimates and outputs $M$ predictions for each point. 

\paragraph{Correlation Volume}
We compute the dot product between image features $\phi_t \in  \mathbb{R}^{d \times \frac{H}{k} \times \frac{W}{k}}$ and tracked features $Q \in  \mathbb{R}^{d \times N}$ across the channel dimension $d$.
$\langle\,\phi_t, Q^T \rangle \in  \mathbb{R}^{N \times \frac{H}{k} \times \frac{W}{k}}$

We bi-linearly sample from the dot product in the spatial neighbourhood of our current trajectory estimates $(\hat x + \delta, \hat y + \delta), \delta \in [-\Delta,.., \Delta]$ at 4 different scales:

$\hat{C}^{(m)}_{t} = Sample\big (\langle\,\phi_t, Q^T \rangle, (\hat x_t + \delta, \hat y_t + \delta)\big ) \in \mathbb{R}^{N \times  4(2\Delta+1)}   $ 

\paragraph{Visibility and Tracking masks}
We assume that all the points are visible on the first sliding window. 

\paragraph{Transformer}
We process points jointly

The model also updates tracked features for every sliding window to compensate for changes in appearance from the frame where we sampled them.

$\hat P^{(m+1)}, \hat Q^{(m+1)} = Transformer\big (\hat P^{(m)}, \hat Q^{(m)}, emb(\hat P^{(m)}-\hat P^{(m)}_0), \hat{C}^{(m)}, \hat v^{(m)}, \big )$

\subsection{Training}
\paragraph{Unrolled training}
We train the model on sequences of size $T$ in an unrolled fashion with a sliding windows of size $S = 2k, 1 \leq k \leq T/2 $ .
Then the number of sliding windows in a video is: $J = \ceil[\big]{T/\frac{S}{2} - 1}$

\paragraph{Supervision}
We supervise the model with two losses. The first loss is computed over all the predicted coordinates for all the sliding windows:
\begin{equation}
    \mathcal{L}(\hat{P}, P) = \sum_{j=0}^{J-1} {\sum_{t=1}^{S} { \sum_{m=1}^{M} \gamma^{M-m} \|\hat{P}_{\frac{S}{2}*j+t}^{(m)}  - P_{\frac{S}{2}*j+t}\|}},
  \label{eq:also-important}
\end{equation}
where $\gamma=0.8$ and $P$ is the ground truth trajectory.

\subsection{Inference}
