# Supplementary material for: CoTracker: It is Better to Track Together
Source: arXiv:2307.07635 source file (2024-10-01)
Supplement: Supplementary file 2 [file tab_suppl_train_data.tex]

\begin{table*}[t]
\centering
\footnotesize
\caption{  \textbf{Training data}.  }\label{tab:tab_train_data_comparison}
\begin{tabular}{ llccccccccc }
\toprule
\multirow{2}{*}{Method} & \multirow{2}{*}{Training data}  & \multicolumn{3}{c}{TAP-Vid Davis} & \multicolumn{3}{c}{TAP-Vid Kinetics} & \multicolumn{2}{c}{BADJA} \\
\cmidrule(lr){3-5}
\cmidrule(lr){6-8}
& &  AJ & \!\!\!$< \delta^x_{avg}$\! & OA  & AJ & \!\!\!$< \delta^x_{avg}$ & OA & \!\!seg-based\!\! & \!\!3px acc\!\! \\
\midrule

PIPs~\cite{pips} & Flying things++ & 42.2 & 64.8 & 77.7 & 31.7 & 53.7 & 72.9 & 61.9 & 13.5 \\

PIPs~\cite{pips} & TAP-Vid-Kubric  & 43.8 & 66.5 & 77.4 & 32.7 & 55.1 & 72.9 & 64.0 & 14.7 \\
PIPs~\cite{pips} & Dynamic Replica   & 39.7 & 61.5 &  &  &  & & 59.6 &  12.4 \\

\method (Ours)\!\!\! & TAP-Vid-Kubric              & \textbf{51.2} & \textbf{68.5} & \textbf{85.2} & \textbf{43.3} & \textbf{61.4} & \textbf{83.3} & \textbf{65.5} & \textbf{15.4} \\
\method (Ours)\!\!\! & Dynamic Replica    & & & & & & &      62.8    & 16.6 \\

\bottomrule
\end{tabular}

\end{table*}
